# Supplementary material for: Observation of Antiferromagnetic Magnon Pseudospin Dynamics and the Hanle effect
Source: arXiv:2008.00440 ancillary file (2020-12-13)
Supplement: Supplementary file 1 [file Supplemental_Material.pdf]

# Supplementary Information: Observation of Antiferromagnetic Magnon Pseudospin Dynamics and Hanle Effect

T. Wimmer,[1,2,*] A. Kamra,[3] J. Gückelhorn,[1,2] M. Opel,[1]
S. Geprägs,[1] R. Gross,[1,2,4] H. Huebl,[1,2,4] and M. Althammer[1,2,†]

[1] *Walther-Meißner-Institut, Bayerische Akademie der Wissenschaften, 85748 Garching, Germany*
[2] *Physik-Department, Technische Universität München, 85748 Garching, Germany*
[3] *Center for Quantum Spintronics, Department of Physics, Norwegian University of Science and Technology, NO-7491 Trondheim, Norway*
[4] *Munich Center for Quantum Science and Technology (MCQST), Schellingstr. 4, D-80799 München, Germany*

(Dated: October 2, 2020)

* tobias.wimmer@wmi.badw.de
† matthias.althammer@wmi.badw.de

## I. HEMATITE THIN FILMS AND MAGNETOMETRY MEASUREMENTS

The $t = 15\,\text{nm}$ thick, single crystalline (0001)-oriented hematite ($\alpha$-$Fe_2O_3$) film was grown via pulsed laser deposition at the Walther-Meißner-Institut on a (0001)-oriented sapphire ($Al_2O_3$) substrate using a substrate temperature of 320 °C, an oxygen pressure of 25 µbar, a laser fluence at the target of $2.5\,\text{J/cm}^2$ and a repetition rate of 2 Hz.

In bulk crystals, hematite exhibits a Néel temperature of $T_\text{N} = 953\,\text{K}$ and undergoes a spin reorientation, the so-called Morin transition, at $T_\text{M} \approx 263\,\text{K}$ [S1, S2]. This transition is characterized by a sign change of the uniaxial magnetic anisotropy, resulting in a transition from a magnetic easy (0001)-plane above $T_\text{M}$ to a magnetic easy (0001)-axis below $T_\text{M}$. As suggested from our magnon transport data presented in the main text, our hematite thin films are characterized by a finite magnetic moment in the (0001)-plane over the whole measured temperature range from 100 K to 300 K. In particular, this indicates the absence of the Morin transition expected from bulk crystals. To verify this magnetic behaviour, we performed SQUID (superconducting quantum interference device) magnetometry using a 90 nm-thick film (to ensure a larger magnetic moment as compared to the thin film used in the main text), which was prepared with the same parameters as the film used in the main text. The measured magnetic moment in the (0001)-plane is shown as a function of the in-plane magnetic field in Fig. S1 for several temperatures. For each measurement, a linear (diamagnetic) background was subtracted from the data. Clearly, the data shows a finite magnetic moment as well as a hysteretic behaviour. This finding supports the finite canting of the sublattice moments, which is only present for $T > T_\text{M}$ (above the Morin-transition) due to the perpendicular configuration of the in-plane oriented magnetic sublattice spins and the out-of-plane oriented DMI vector [S2]. The hysteretic behaviour can be explained by the three-fold easy-plane anisotropy due to the hexagonal crystal structure [S2], leading to the formation of 120° domain walls [S3, S4]. As described in the main text, increasing magnetic fields $\mu_0 H$ lead to a growth of domains with a perpendicular orientation of their Néel vector $\mathbf{n}$ to $\mathbf{H}$ with a monodomainization field of $H_\text{MD} = 600\,\text{mT}$ [S4]. This monodomainization field agrees reasonably well with our magnetic hysteresis curve, exhibiting a closure of the hysteresis at approximately 700 mT. Hence, the measured hysteresis behaviour supports the expected domain configuration of the hematite above the Morin transition [S5, S6].

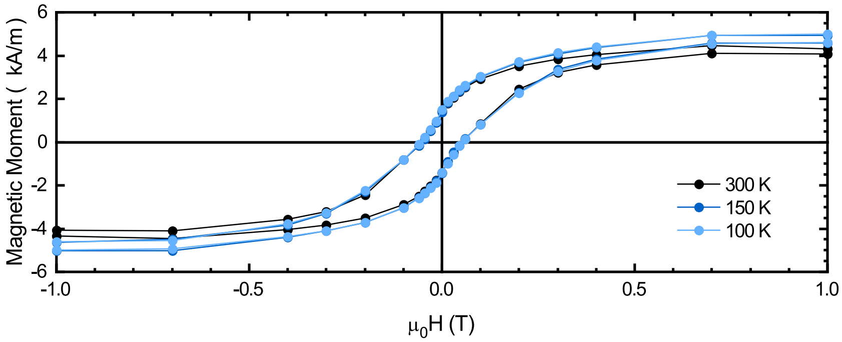


FIG. S1. In-plane SQUID magnetometry measurement of a 90 nm-thick film of (0001)-oriented hematite. The magnetic hysteresis curves are recorded for different temperatures. Clearly, we observe the weak ferromagnetic moment corresponding to the small canting of the magnetic sublattices above $T_\text{M}$.

Different to the expected behaviour of bulk hematite, we do not observe any indication of a Morin transition in the temperature range from 100 K to 300 K. This feature is not yet entirely clear. However, recent reports indicate a strong decrease (up to a complete absence) of the Morin transition temperature $T_\text{M}$ for thin film hematite [S7, S8], which might be related to a strain-induced change of the magnetic anisotropy.

## II. ALL-ELECTRICAL MAGNON TRANSPORT EXPERIMENTS

For the injection and detection of magnons in the hematite, platinum (Pt) electrodes with a thickness of 5 nm were deposited via DC magnetron sputtering and patterned into strips of lengths $l = 162\,\mu\text{m}$ (injector) and $l = 148\,\mu\text{m}$ (detector) via electron beam lithography. Subsequently, an Al layer of 50 nm is deposited on the film by DC sputtering and patterned into leads for the Pt strips to contact the device electrically. For the measurements shown in the main text, DC current densities in the order of $2 \times 10^{11}\,\text{A}\,\text{m}^{-2}$ are fed through the injector strips with a Keithley 2400 current source. To detect the magnon spin signal, we measure the voltage signals at the detectors using a Keithley 2182 nanovoltmeter. Each of the structures studied in this work have a constant detector width of $w_\text{det} = 500\,\text{nm}$ and edge-to-edge distances of either $d_\text{edge} = 200\,\text{nm}$ or $d_\text{edge} = 400\,\text{nm}$. The injector widths vary from $w_\text{inj} = 200\,\text{nm}$

to $w_{\text{inj}} = 800\,\text{nm}$. In the main text, we use the center-to-center distance between the strips to describe the effective transport length $d$. A charge current $I_{\text{inj}}$ is applied to the injector and the electrical voltage contribution $V^{\text{el}}_{\text{det}}$ is measured. The electrical and thermal contributions are separated by the current reversal method [S9, S10]. With this method, it is possible to discern electrical and thermal effects by their symmetry, since electrical (thermal) effects are antisymmetric (symmetric) under inversion of current polarity. In order to compare between different geometries and injector currents $I_{\text{inj}}$, we define the normalized magnon spin signal $R^{\text{el}}_{\text{det}} = (V^{\text{el}}_{\text{det}}/I_{\text{inj}}) \cdot (A_{\text{inj}}/A_{\text{det}})$ , where $A_{\text{inj}}$ and $A_{\text{det}}$ are the interface areas at the injector and detector, respectively.

## III. FITTING PROCEDURE FOR FIELD-DEPENDENT MAGNON TRANSPORT DATA

The fitting function of our field-dependent magnon spin signals $\Delta R^{\text{el}}_{\text{det}}$ plotted in Figs. 1(e) and 3(a) of the main text reads

$$\Delta R^{\text{el}}_{\text{det}}(\mu_0 H) = R_0 + C s(z), \tag{S1}$$

where $R_0$ accounts for a finite offset signal and $C$ constitutes a constant scaling parameter to take into account the conversion effects from the magnon spin density $s(z)$ [taken from Eq. (3) of the main text, which is rigorously derived in Secs. VI B and VI C, see Eq. (S8)] to the measured detector signal $\Delta R^{\text{el}}_{\text{det}}$. Regarding the fitting routine, we choose the free parameters to be $R_0$, $D$, $\tau_{\text{s}}$ and $\tilde{\omega}_{\text{an}}$. Furthermore, the product $C \cdot j_{\text{s0}}$ is treated as a single fitting parameter. Assuming $m_{\text{net}} = m_{\text{net0}} + \chi H$, with $\chi$ the susceptibilty of easy-plane hematite and $m_{\text{net0}}$ the net magnetic moment at zero external magnetic field due to the DMI, the equivalent magnetic moment $\tilde{m}$ defined in Eq. (2) of the main text (see also Eq. (S33) in this Supplemental) can be expressed as $\tilde{m} = \chi H_{\text{DMI}} = m_{\text{net0}}$. Hence, we treat $\tilde{m}$ as a fixed parameter in the fit using the bulk value $m_{\text{net0}} = 2.1 \times 10^{-25}\,\text{A}\,\text{m}^2$ taken from Ref. [S11].

## IV. TEMPERATURE DEPENDENCE OF THE MAXIMUM SIGNAL RESPONSE

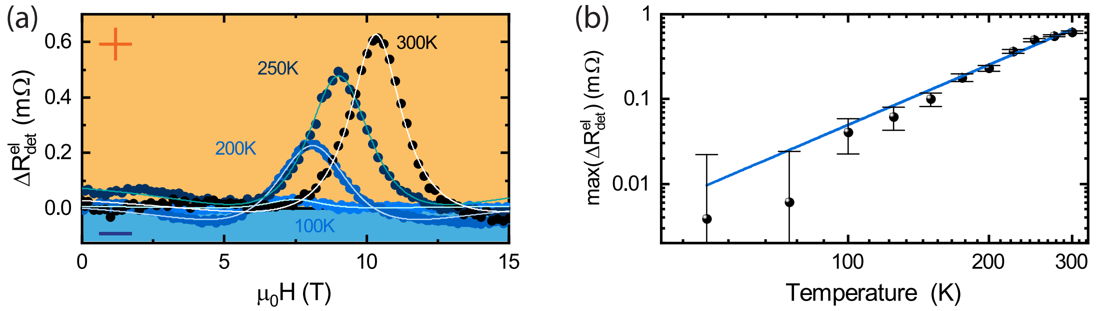


FIG. S2. (a) Field-dependent magnon transport signals for various temperatures taken from the main text Figure 3(a). (b) Temperature dependence of the maximum signal max($\Delta R^{\text{el}}_{\text{det}}$) extracted at the compensation field $\mu_0 H_{\text{c}}$ for each temperature from panel (a). The solid blue line is a fit to a power law dependence, suggesting $\propto T^{2.36}$.

For a more detailed investigation of the magnon transport signals we study the temperature dependence of the maximum signal amplitudes. For convenience, we plot the field-dependent magnon transport signals from the main text (Fig. 3(a)) again in Fig. S2(a). We then extract the maximum signal amplitudes max($\Delta R^{\text{el}}_{\text{det}}$), evaluated at the compensation field $\mu_0 H_{\text{c}}$, for each temperature and plot the result in Fig. S2(b). Fitting the data with a simple power law dependence of the form $R^{\text{el}}_{\text{det},0} T^n$, we find $n = 2.36$ (blue solid line in Fig. S2(b)). This agrees reasonably well with theoretical results that predict a temperature dependence of $\propto T^2$ for the electron spin to magnon conversion at a HM/AFI interface [S12], verifying once more that the transport is indeed due to pure magnon currents. The slight discrepancy between theory and our data most probably stems from addtional temperature dependencies due to the transport of the magnons, which is not included in the spin to magnon interface conversion parameter of Ref. S12.

## V. CURRENT-VOLTAGE CHARACTERISTICS AND CROSSTALK BETWEEN INJECTOR AND DETECTOR

In this Section, we verify the linearity of the magnon transport signals as a function of the injector current $I_{\text{inj}}$. For this purpose, we apply a field corresponding to the compensation field $\mu_0 H_{\text{c}}$ along the length of the Pt electrodes to

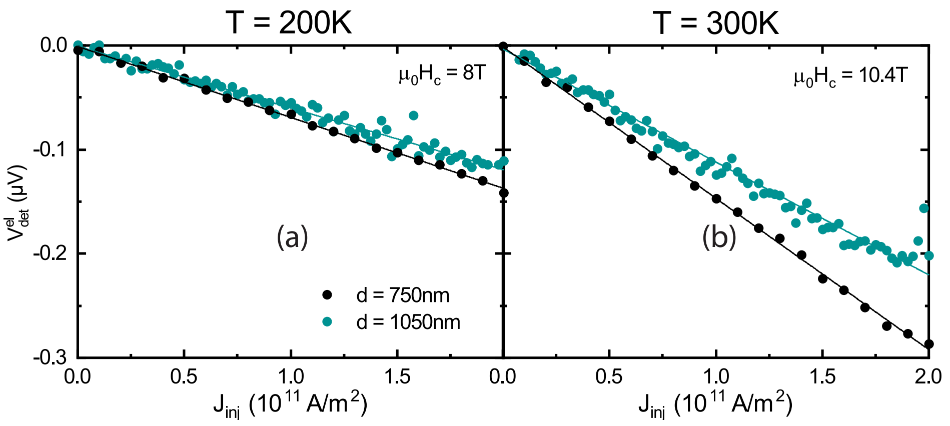


FIG. S3. (a) Current-voltage characteristic measured at $T = 200\,\mathrm{K}$ at the corresponding compensation field $\mu_0 H_c = 8\,\mathrm{T}$ applied along the length of the Pt electrodes. (b) Current-voltage characteristic measured at $T = 300\,\mathrm{K}$ at the corresponding compensation field $\mu_0 H_c = 10.4\,\mathrm{T}$. Both panels show the data for two different devices with $d = 750\,\mathrm{nm}$ and $d = 1050\,\mathrm{nm}$. Solid lines are linear fits to the data.

ensure the maximum signal response. The corresponding measurement of the detector voltage $V_{\mathrm{det}}^{\mathrm{el}}$ as a function of the current density $J_{\mathrm{inj}} = \frac{I_{\mathrm{inj}}}{t_{\mathrm{Pt}} \cdot w_{\mathrm{inj}}}$ in the injector is shown in Fig. S3 (a) for two different injector-detector distances $d$ at a temperature $T = 200\,\mathrm{K}$. The same measurement is repeated at a temperature $T = 300\,\mathrm{K}$ and shown in Fig. S3 (b). Each device shows a clear linear behaviour as a function of the injector current, as expected from the magnon transport effect [S13, S14]. The solid lines correspond to linear fits of the data.

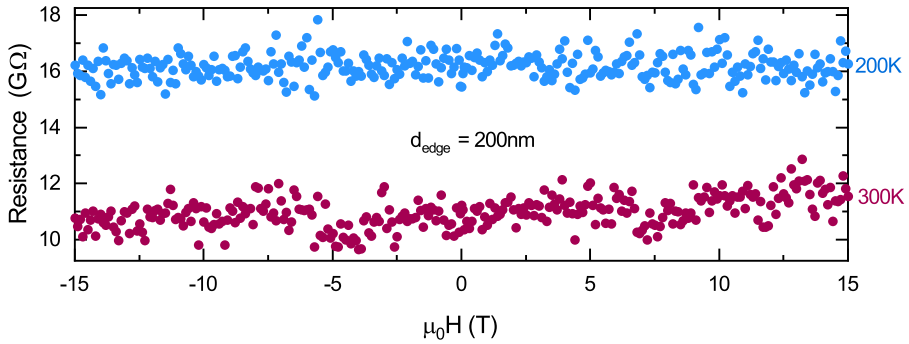


FIG. S4. Resistance as a function of magnetic field (applied along the length of the Pt electrodes) measured between an injector and detector electrode with an edge-to-edge distance $d_{\mathrm{edge}} = 200\,\mathrm{nm}$ for two different temperatures $T = 300\,\mathrm{K}$ and $T = 200\,\mathrm{K}$.

Last but not least, we check the insulating nature of the hematite thin film. Thus, we apply a constant voltage of $V_{\mathrm{cross}} = 5\,\mathrm{V}$ between the injector and detector electrode and measure the corresponding current $I_{\mathrm{cross}}$. In Fig. S4, the resistance is calculated as $V_{\mathrm{cross}}/I_{\mathrm{cross}}$ and is plotted as a function of the external magnetic field applied along the length of the Pt electrodes for two different temperatures. The measured device exhibits an edge-to-edge distance of $d = 200\,\mathrm{nm}$. As evident from the data, we observe a highly insulating resistance with a minimum value of $\sim 10\,\mathrm{G\Omega}$ at the highest measured temperature of $T = 300\,\mathrm{K}$. As expected, the resistance even increases to $\sim 16\,\mathrm{G\Omega}$ when lowering the temperature to $T = 200\,\mathrm{K}$. Due to the good insulating behaviour of our hematite, we can exclude any spurious contribution to the electrical magnon transport signal, as e.g. an antiferromagnetic anisotropic magnetoresistance from the hematite itself.

## VI. DIFFUSIVE MAGNONIC SPIN TRANSPORT WITH COHERENT PSEUDOSPIN PRECESSION

In this section, we formulate a description for magnon spin transport in the diffusive limit relevant for typical experiments [S13, S14]. Building upon previous formulations [S15–S17] and formal similarity between electron spin

and antiferromagnetic magnon pseudospin [S18–S20], we obtain the corresponding spin transport equation including the coherent dynamics of the eigenmodes captured via pseudospin precession [S21]. This allows us to evaluate the spatial profile of the nonequilibrium spin density, and thus the magnon spin signal defined in the main text, in the antiferromagnet resulting from spin current injection via the platinum electrode.

### A. Diffusive magnonic spin transport without pseudospin dynamics

Uniformly ordered magnetic insulators host bosonic collective excitations - magnons - that carry spin in directions collinear with the order parameter. For ferromagnets, magnon excitations may be described by a Hamiltonian: $\tilde{H}_{\mathrm{FI}} = \sum_{\boldsymbol{k}} \hbar\omega_{\boldsymbol{k}} \tilde{a}^\dagger_{\boldsymbol{k}} \tilde{a}_{\boldsymbol{k}}$ and carry spin angular momentum pointing along the magnetization vector. On the other hand, bipartite antiferromagnets are comprised by two interpenetrating magnetic sublattices with antiparallel magnetizations. Therefore, under certain general conditions to be discussed later, they host pairs of magnonic excitations described by $\tilde{H}_{\mathrm{AF}} = \sum_{\boldsymbol{k}} \hbar\omega_{\boldsymbol{k}} (\tilde{\alpha}^\dagger_{\boldsymbol{k}} \tilde{\alpha}_{\boldsymbol{k}} + \tilde{\beta}^\dagger_{\boldsymbol{k}} \tilde{\beta}_{\boldsymbol{k}})$ carrying spin in the two antiparallel directions collinear with the Néel vector. For both kinds of magnets in a broad parameter regime, magnons mediate a diffusive spin transport [S15–S17] through the magnetic insulator that can be described by the typical diffusion equation:

$$\frac{\partial s}{\partial t} = D \boldsymbol{\nabla}^2 s - \frac{s}{\tau_s}, \tag{S2}$$

where $s$ is the nonequilibrium spin density, $D$ is the diffusion constant, and $\tau_s$ is the spin relaxation time. Here, $s$ is a scalar corresponding to spin along the order parameter as discussed above. $D$ and $\tau_s$ are obtained by averaging over the occupied magnon modes.

### B. Diffusive magnonic spin transport with pseudospin dynamics

When the magnetic energy landscape is not axially symmetric about the order parameter direction, the spin-up and -down magnon modes in an antiferromagnetic insulator (AFI) become coherently coupled [S22, S23] as described by

$$\tilde{H}_{\mathrm{AF}} = \sum_{\boldsymbol{k}} \hbar\omega_{\boldsymbol{k}} (\tilde{\alpha}^\dagger_{\boldsymbol{k}} \tilde{\alpha}_{\boldsymbol{k}} + \tilde{\beta}^\dagger_{\boldsymbol{k}} \tilde{\beta}_{\boldsymbol{k}}) + \frac{\hbar \bar{\Omega}_{\boldsymbol{k}}}{2} (\tilde{\alpha}^\dagger_{\boldsymbol{k}} \tilde{\beta}_{\boldsymbol{k}} + \tilde{\alpha}_{\boldsymbol{k}} \tilde{\beta}^\dagger_{\boldsymbol{k}}), \tag{S3}$$

where $\bar{\Omega}_{\boldsymbol{k}}$ describes the coherent coupling frequency. Such an axial-symmetry breaking may result from any spin-nonconserving interaction [S22] such as dipolar fields [S20, S22], magnetocrystalline anisotropy [S24], and Dzyaloshinskii-Moriya interaction (DMI) [S19, S25]. This coherent effect of spin-nonconserving interactions is distinct from their role in causing an incoherent loss of spin current that determines $\tau_s$ in Eq. (S2). The effect of this coherent coupling is to result in new magnonic eigenmodes formed by equal superpositions of spin-up and -down magnons. These new excitations, therefore, carry zero average spin [S22]. However, in certain nonequilibrium situations such as the non-local spin transport under investigation, it is more convenient to continue working in the basis of spin-up and -down magnons treating the $\bar{\Omega}_{\boldsymbol{k}}$ contribution perturbatively. We adopt this approach here and discuss it in detail elsewhere [S21].

The spin-up and -down magnon modes of AFIs constitute a two-level system similar to a conduction electron with its spin-up and -down states [S18–S20, S26]. A general state of the electron is described by a coherent superposition between its spin-up and -down states. The resultant state is associated with a vector on the Bloch sphere, which becomes the expectation value of the electron spin. More generally, a superposition between any two states can be described by an analogous vector on the Bloch sphere. Due to its formal similarity to the electron spin case, this vector is often called pseudospin. Following this formal equivalence between AFI magnons and electron spin states, we associate the magnonic excitations with a pseudospin vector, as discussed in the main text. Within our chosen convention, the z-component of pseudospin is identified with the actual magnonic spin and is directly probed in our experiments.

Exploiting the similarity between electronic spin [S27] and magnonic pseudospin transport and dynamics, the nonequilibrium pseudospin density $\boldsymbol{\mathcal{S}}$ can be described as [S21]:

$$\frac{\partial \boldsymbol{\mathcal{S}}}{\partial t} = D \boldsymbol{\nabla}^2 \boldsymbol{\mathcal{S}} - \frac{\boldsymbol{\mathcal{S}}}{\tau_s} + \boldsymbol{\mathcal{S}} \times \Omega\, \hat{\boldsymbol{y}}, \tag{S4}$$

where $\Omega = \langle \bar{\Omega}_{\boldsymbol{k}} \rangle$ averaged over the occupied magnon modes accounts for the coherent pseudospin dynamics. As mentioned above, the spin density is given by the z component of the pseudospin density, i.e. $s = \mathcal{S}_z$. For $\Omega = 0$, Eq. (S4) reduces to Eq. (S2) consistent with spin transport mediated by uncoupled magnonic excitations.

### C. Spin transport through a thin film channel

In the following analysis, we consider the equilibrium Néel order and spin injection/detection via the metal electrode to be collinear with $\hat{\boldsymbol{z}}$. Thus, we implicitly assume the noncollinearity in our AFI to be negligibly small. This is consistent with exchange interaction being much stronger than other energy contributions in the AFI and will be demonstrated explicitly in the next section.

In order to obtain the spatial profile of the nonequilibrium spin injected into our thin AFI film, we solve Eq. (S4) in steady state:

$$D\mathcal{S}_x'' - \frac{\mathcal{S}_x}{\tau_s} - \mathcal{S}_z\Omega = 0, \tag{S5}$$

$$D\mathcal{S}_z'' - \frac{\mathcal{S}_z}{\tau_s} + \mathcal{S}_x\Omega = 0, \tag{S6}$$

where the pseudospin density $\boldsymbol{\mathcal{S}}$ has been assumed to vary only with $z$ in accordance with our device design and dimensions. Considering a spin current polarized along z-direction $j_{s0}$ injected at $z = 0$, the boundary conditions become $-D\partial\mathcal{S}_z/\partial z|_{z=0} = j_{s0}$ and $\partial\mathcal{S}_x/\partial z|_{z=0} = 0$, the desired solution is obtained after some algebra:

$$\mathcal{S}_x = -\frac{j_{s0}\lambda_s}{D(a^2+b^2)} e^{-\frac{az}{\lambda_s}} \left( b\cos\left(\frac{bz}{\lambda_s}\right) + a\sin\left(\frac{bz}{\lambda_s}\right)\right), \tag{S7}$$

$$\mathcal{S}_z = \frac{j_{s0}\lambda_s}{D(a^2+b^2)} e^{-\frac{az}{\lambda_s}} \left( a\cos\left(\frac{bz}{\lambda_s}\right) - b\sin\left(\frac{bz}{\lambda_s}\right)\right), \tag{S8}$$

where $\lambda_s \equiv \sqrt{D\tau_s}$ is the spin relaxation length and

$$a \equiv \frac{1}{\sqrt{2}}\sqrt{1 + \sqrt{1+\Omega^2\tau_s^2}}, \tag{S9}$$

$$b \equiv \frac{1}{\sqrt{2}}\sqrt{-1 + \sqrt{1+\Omega^2\tau_s^2}}. \tag{S10}$$

Here, Eq. (S8) describes the nonequilibirum spin density in the AFI. Further, in the limit of weak coupling with the detector electrode, the voltage detected, corresponding to the magnon spin signal, is directly proportional to $s(z) = \mathcal{S}_z(z)$ from Eq. (S8) [S15].

## VII. COHERENT COUPLING FREQUENCY

In the present section, we relate the coherent coupling frequency $\Omega$ [Eq. (S4)] with the various contributions to the magnetic energy landscape of our AFI. To this end, we employ a simplified minimal model motivated by the macroscopic free energy density for hematite [S2] that allows us to capture the key phenomena and dependencies satisfactorily. In this manner, we obtain the full magnon Hamiltonian. Considering that the exchange interaction in the AFI is much stronger than the remaining energy contributions, we treat the coupling between spin-up and -down magnons perturbatively. This allows us to obtain an analytic expression for the desired coupling frequency.

### A. Spin Hamiltonian

Disregarding a weak in-plane anisotropy, our hematite thin film may qualitatively be described via the following spin Hamiltonian [S2]:

$$\tilde{H}_{\rm AFI} = \tilde{H}_{\rm Z} + \tilde{H}_{\rm ex} + \tilde{H}_{\rm an} + \tilde{H}_{\rm DMI}, \tag{S11}$$

accounting for contributions from Zeeman energy, exchange, easy-plane anisotropy, and DMI given by

$$\tilde{H}_{\mathrm{Z}} = \mu_0|\gamma|H\sum\left[\tilde{S}_{1y}(\boldsymbol{r}_i)+\tilde{S}_{2y}(\boldsymbol{r}_j)\right], \tag{S12}$$

$$\tilde{H}_{\mathrm{ex}} = \frac{J}{\hbar^2}\sum_{<i,j>}\tilde{\boldsymbol{S}}_1(\boldsymbol{r}_i)\cdot\tilde{\boldsymbol{S}}_2(\boldsymbol{r}_j), \tag{S13}$$

$$\tilde{H}_{\mathrm{an}} = \frac{K}{\hbar^2}\sum\left[\left(\tilde{S}_{1x}(\boldsymbol{r}_i)\right)^2+\left(\tilde{S}_{2x}(\boldsymbol{r}_j)\right)^2\right], \tag{S14}$$

$$\tilde{H}_{\mathrm{DMI}} = \frac{\mathcal{D}}{\hbar^2}\sum_{<i,j>}\hat{\boldsymbol{x}}\cdot\left[\tilde{\boldsymbol{S}}_1(\boldsymbol{r}_i)\times\tilde{\boldsymbol{S}}_2(\boldsymbol{r}_j)\right]. \tag{S15}$$

Here, $\tilde{\boldsymbol{S}}_1(\boldsymbol{r}_i)$ and $\tilde{\boldsymbol{S}}_2(\boldsymbol{r}_j)$ are the operators for spins on sublattices 1 and 2, respectively with $< i, j >$ denoting pairs of nearest neighbors. $H$ is the external field applied along y-direction, $\gamma$ $(< 0)$ is the gyromagnetic ratio for each sublattice, and $J$, $K$, and $\mathcal{D}$ are positive constants that respectively parameterize the exchange, anisotropy, and DMI contributions.

The various contributions to the spin Hamiltonian Eq. (S11) capture distinct effects in the AFI [S2]. The exchange interaction prefers the two sublattice spins to be aligned antiparallel to each other. It is the strongest energy scale in the system. The Zeeman contribution tries to align the total magnetic moment along the applied field. This results in the individual sublattice magnetizations aligning orthogonal to the field and subtending a small, field-dependent canting angle $\phi$ instead of the perfect antiparallel alignment desired by exchange. The anisotropy in the present case prefers the sublattice spins to stay in the y-z plane. The DMI works against the exchange and prefers to orient the two sublattice spins orthogonal to each other. Its effect on the equilibrium state is to cause canting between the two sublattice spins similar to the applied magnetic field.

## B. Magnon Hamiltonian

Based on a qualitative understanding of the various energy contributions [Eq. (S11)], we assume a canted equilibrium state with the net spin order parameter for sublattices 1 and 2 directed along $\cos\phi\,\hat{\boldsymbol{z}}-\sin\phi\,\hat{\boldsymbol{y}}$ and $-\cos\phi\,\hat{\boldsymbol{z}}-\sin\phi\,\hat{\boldsymbol{y}}$. Here, the spin points opposite to the magnetic moment due to the negative gyromagnetic ratio and the canting angle $\phi$ $(\ll 1)$ is to be determined based on the condition for equilibrium.

In order to examine excitations, Eq. (S11) needs to be linearized about the assumed equilibrium configuration via Holstein-Primakoff transformation. To this end, we define a new primed coordinate system obtained via a rotation by angle $\phi$ about the x-axis such that the sublattice 1 spin order points along $\hat{\boldsymbol{z}}'$. Another double primed coordinate system obtained via an opposite rotation about the x-axis enables sublattice 2 spin order to point along $-\hat{\boldsymbol{z}}''$. Employing these coordinate systems, the Holstein-Primakoff transformation for the canted system become:

$$\tilde{S}_{1+}(\boldsymbol{r}_i)=\hbar\sqrt{2S}\;\tilde{a}_i,\quad \tilde{S}_{1-}(\boldsymbol{r}_i)=\hbar\sqrt{2S}\;\tilde{a}_i^\dagger,\quad \tilde{S}_{1z'}(\boldsymbol{r}_i)=\hbar(S-\tilde{a}_i^\dagger\tilde{a}_i), \tag{S16}$$

$$\tilde{S}_{2+}(\boldsymbol{r}_j)=\hbar\sqrt{2S}\;\tilde{b}_j^\dagger,\quad \tilde{S}_{2-}(\boldsymbol{r}_j)=\hbar\sqrt{2S}\;\tilde{b}_j,\quad \tilde{S}_{2z''}(\boldsymbol{r}_j)=\hbar(-S+\tilde{b}_j^\dagger\tilde{b}_j), \tag{S17}$$

where $\tilde{S}_{1\pm}=\tilde{S}_{1x}\pm i\tilde{S}_{1y'}$ and $\tilde{S}_{2\pm}=\tilde{S}_{2x}\pm i\tilde{S}_{2y''}$. $\tilde{a}_i$ and $\tilde{b}_j$ are the magnon annihilation operators on sublattices 1 and 2, respectively.

Expressing the spin Hamiltonian [Eq. (S11)] in the new coordinate systems, employing the Holstein-Primakoff transformation [Eqs. (S16) and (S17)] for our canted system, and switching to Fourier space, we obtain the magnon Hamiltonian:

$$\tilde{H}_{\mathrm{mag}}=\sum_{\boldsymbol{k}}\left[A_{\boldsymbol{k}}\tilde{a}_{\boldsymbol{k}}^\dagger\tilde{a}_{\boldsymbol{k}}+B_{\boldsymbol{k}}\tilde{b}_{\boldsymbol{k}}^\dagger\tilde{b}_{\boldsymbol{k}}+\left(C_{\boldsymbol{k}}\tilde{a}_{\boldsymbol{k}}\tilde{b}_{-\boldsymbol{k}}+\mathrm{h.c.}\right)+\left(D_{\boldsymbol{k}}\tilde{a}_{\boldsymbol{k}}\tilde{a}_{-\boldsymbol{k}}+E_{\boldsymbol{k}}\tilde{b}_{\boldsymbol{k}}\tilde{b}_{-\boldsymbol{k}}+\mathrm{h.c.}\right)+\left(F_{\boldsymbol{k}}\tilde{a}_{\boldsymbol{k}}\tilde{b}_{\boldsymbol{k}}^\dagger+\mathrm{h.c.}\right)\right], \tag{S18}$$

where

$$A_{\boldsymbol{k}}=B_{\boldsymbol{k}}\approx JSZ+KS, \tag{S19}$$

$$C_{\boldsymbol{k}}\approx JSZ\gamma_{\boldsymbol{k}}, \tag{S20}$$

$$D_{\boldsymbol{k}}=E_{\boldsymbol{k}}=\frac{KS}{2}, \tag{S21}$$

$$F_{\boldsymbol{k}}=\phi\mathcal{D}SZ\gamma_{\boldsymbol{k}}. \tag{S22}$$

In the equations above, terms to the lowest order in $1/J$ have been retained. $Z$ is the number of nearest neighbors, $\gamma_{\boldsymbol{k}} = (1/Z)\sum_{\boldsymbol{\delta}} e^{i\boldsymbol{k}\cdot\boldsymbol{\delta}}$ with $\boldsymbol{\delta}$ running over nearest neighbors. Further, $\phi = (\hbar\mu_0|\gamma|H - \mathcal{D}SZ)/(2JSZ) \ll 1$ has been determined from the equilibrium condition.

### C. Perturbative evaluation of coupling frequency

While the magnon Hamiltonian [Eq. (S18)] obtained in the previous subsection can be diagonalized exactly [S22, S23], the exact solution is unwieldy and does not help our present goal. Thus, we invoke the hierarchy of interactions to split our problem [S28] into an unperturbed Hamiltonian $\tilde{H}_{\text{base}}$ and a perturbation $\tilde{H}_{\text{coup}}$. Here, the unperturbed base Hamiltonian includes terms that bear contributions from the exchange interaction:

$$\tilde{H}_{\text{base}} = \sum_{\boldsymbol{k}} \left[ A_{\boldsymbol{k}} \left( \tilde{a}^{\dagger}_{\boldsymbol{k}} \tilde{a}_{\boldsymbol{k}} + \tilde{b}^{\dagger}_{\boldsymbol{k}} \tilde{b}_{\boldsymbol{k}} \right) + \left( C_{\boldsymbol{k}} \tilde{a}_{\boldsymbol{k}} \tilde{b}_{-\boldsymbol{k}} + \text{h.c.} \right) \right], \tag{S23}$$

$$= \sum_{\boldsymbol{k}} \hbar\omega_{\boldsymbol{k}} \left( \tilde{\alpha}^{\dagger}_{\boldsymbol{k}} \tilde{\alpha}_{\boldsymbol{k}} + \tilde{\beta}^{\dagger}_{\boldsymbol{k}} \tilde{\beta}_{\boldsymbol{k}} \right), \tag{S24}$$

where $\hbar\omega_{\boldsymbol{k}} = \sqrt{A_{\boldsymbol{k}}^2 - C_{\boldsymbol{k}}^2}$ and the base Hamiltonian has been diagonalized via a Bogoliubov transformation [S28]:

$$\tilde{\alpha}_{\boldsymbol{k}} = u_{\boldsymbol{k}} \tilde{a}_{\boldsymbol{k}} + v_{\boldsymbol{k}} \tilde{b}^{\dagger}_{-\boldsymbol{k}}, \quad \tilde{\beta}_{\boldsymbol{k}} = u_{\boldsymbol{k}} \tilde{b}_{\boldsymbol{k}} + v_{\boldsymbol{k}} \tilde{a}^{\dagger}_{-\boldsymbol{k}}, \tag{S25}$$

$$u_{\boldsymbol{k}} = \sqrt{\frac{A_{\boldsymbol{k}} + \hbar\omega_{\boldsymbol{k}}}{2\hbar\omega_{\boldsymbol{k}}}}, \qquad v_{\boldsymbol{k}} = \sqrt{\frac{A_{\boldsymbol{k}} - \hbar\omega_{\boldsymbol{k}}}{2\hbar\omega_{\boldsymbol{k}}}}. \tag{S26}$$

Thus, the unperturbed base Hamiltonian admits spin-up and -down magnon modes corresponding to the annihilation operators $\tilde{\alpha}_{\boldsymbol{k}}$ and $\tilde{\beta}_{\boldsymbol{k}}$.

The perturbation Hamiltonian consists of terms that stem from the weaker spin-nonconserving interactions which necessarily underlie the coherent coupling physics under investigation:

$$\tilde{H}_{\text{coup}} = \sum_{\boldsymbol{k}} \left[ D_{\boldsymbol{k}} \left( \tilde{a}_{\boldsymbol{k}} \tilde{a}_{-\boldsymbol{k}} + \tilde{b}_{\boldsymbol{k}} \tilde{b}_{-\boldsymbol{k}} + \text{h.c.} \right) + \left( F_{\boldsymbol{k}} \tilde{a}_{\boldsymbol{k}} \tilde{b}^{\dagger}_{\boldsymbol{k}} + \text{h.c.} \right) \right], \tag{S27}$$

$$= \sum_{\boldsymbol{k}} \left[ 4D_{\boldsymbol{k}} u_{\boldsymbol{k}} v_{\boldsymbol{k}} - F_{\boldsymbol{k}} \left( u_{\boldsymbol{k}}^2 + v_{\boldsymbol{k}}^2 \right) \right] \tilde{\alpha}_{\boldsymbol{k}} \tilde{\beta}^{\dagger}_{\boldsymbol{k}} + \text{h.c.}, \tag{S28}$$

where we invoked the unperturbed Hamiltonian solution and the rotating wave approximation in the last step above [S28]. From Eqs. (S28) and (S3), we obtain:

$$\hbar\bar{\Omega}_{\boldsymbol{k}} = 2KSf(\boldsymbol{k}) - g(\boldsymbol{k})\mathcal{D}\phi SZ, \tag{S29}$$

where $f(\boldsymbol{k}) \equiv 2u_{\boldsymbol{k}} v_{\boldsymbol{k}}$ and $g(\boldsymbol{k}) \equiv 2\gamma_{\boldsymbol{k}}(u_{\boldsymbol{k}}^2 + v_{\boldsymbol{k}}^2)$. The average coupling frequency $\Omega$ that enters Eq. (S4) is obtained by averaging over the occupied magnon modes [S21]:

$$\hbar\Omega = \hbar \left\langle \bar{\Omega}_{\boldsymbol{k}} \right\rangle = \langle g(\boldsymbol{k}) \rangle \left( 2KSl - \mathcal{D}\phi SZ \right), \tag{S30}$$

where $l \equiv \langle f(\boldsymbol{k}) \rangle / \langle g(\boldsymbol{k}) \rangle$. Since $\Omega$ enters the spatial spin profile Eq. (S8) only in combination with $\tau_s$, we can absorb the overall multiplicative constants into the latter. Thus, we have:

$$\hbar\Omega = 2KSl - \mathcal{D}\phi SZ, \tag{S31}$$

$$= 2KSl - \mu_0 H_{\text{DMI}} m_{\text{net}}, \tag{S32}$$

$$= \hbar\tilde{\omega}_{\text{an}} - \mu_0 \tilde{m} H, \tag{S33}$$

where $m_{\text{net}} = 2M_0 V\phi$, $H_{\text{DMI}} = \mathcal{D}SZ/(2M_0 V\mu_0)$, $\hbar\tilde{\omega}_{\text{an}} = 2KSl + \mathcal{D}^2 SZ/(2J) \approx 2KSl$, and $\tilde{m} = \mathcal{D}|\gamma|\hbar/(2J)$ with $M_0$ the saturation magnetization for each sublattice and $V$ the magnet volume. Eqs. (S32) and (S33) constitute the final result of this section and provide the expressions employed in the main manuscript.

---

[S1] F. J. Morin, Phys. Rev. **78**, 819 (1950).

[S2] A. H. Morrish, *Canted Antiferromagnetism: Hematite* (WORLD SCIENTIFIC, 1995).
[S3] R. Nathans, S. J. Pickart, H. A. Alperin, and P. J. Brown, Phys. Rev. **136**, A1641 (1964).
[S4] J. C. Marmeggi, D. Hohlwein, and E. F. Bertaut, Physica Status Solidi (a) **39**, 57 (1977).
[S5] J. A. Eaton and A. H. Morrish, Journal of Applied Physics **40**, 3180 (1969).
[S6] P. J. Besser, A. H. Morrish, and C. W. Searle, Physical Review **153**, 632 (1967).
[S7] A. Ross, R. Lebrun, O. Gomonay, D. A. Grave, A. Kay, L. Baldrati, S. Becker, A. Qaiumzadeh, C. Ulloa, G. Jakob, F. Kronast, J. Sinova, R. Duine, A. Brataas, A. Rothschild, and M. Kläui, Nano Letters **20**, 306 (2020).
[S8] J. Han, P. Zhang, Z. Bi, Y. Fan, T. S. Safi, J. Xiang, J. Finley, L. Fu, R. Cheng, and L. Liu, Nature Nanotechnology , 563 (2020).
[S9] S. T. B. Goennenwein, R. Schlitz, M. Pernpeintner, K. Ganzhorn, M. Althammer, R. Gross, and H. Huebl, Applied Physics Letters **107**, 172405 (2015).
[S10] K. Ganzhorn, S. Klingler, T. Wimmer, S. Geprägs, R. Gross, H. Huebl, and S. T. B. Goennenwein, Applied Physics Letters **109**, 022405 (2016).
[S11] R. A. Lefever, in *Landolt-Börnstein - Group III Condensed Matter* (Springer-Verlag) pp. 8–16.
[S12] K. Chen, W. Lin, C. L. Chien, and S. Zhang, Phys. Rev. B **94**, 054413 (2016).
[S13] L. J. Cornelissen, J. Liu, R. A. Duine, J. B. Youssef, and B. J. van Wees, Nature Physics **11**, 1022 (2015).
[S14] R. Lebrun, A. Ross, S. A. Bender, A. Qaiumzadeh, L. Baldrati, J. Cramer, A. Brataas, R. A. Duine, and M. Kläui, Nature **561**, 222 (2018).
[S15] L. J. Cornelissen, K. J. H. Peters, G. E. W. Bauer, R. A. Duine, and B. J. van Wees, Physical Review B **94**, 014412 (2016).
[S16] K. Shen, Physical Review B **100**, 094423 (2019).
[S17] R. E. Troncoso, S. A. Bender, A. Brataas, and R. A. Duine, Physical Review B **101**, 054404 (2020).
[S18] R. Cheng, M. W. Daniels, J.-G. Zhu, and D. Xiao, Scientific Reports **6**, 24223 (2016).
[S19] M. Kawano and C. Hotta, Phys. Rev. B **99**, 054422 (2019).
[S20] K. Shen, Physical Review Letters **124**, 077201 (2020).
[S21] A. Kamra et al., "Antiferromagnetic magnon pseudospin: dynamics and diffusive transport," unpublished.
[S22] A. Kamra, U. Agrawal, and W. Belzig, Phys. Rev. B **96**, 020411 (2017).
[S23] S. M. Rezende, A. Azevedo, and R. L. Rodríguez-Suárez, Journal of Applied Physics **126**, 151101 (2019).
[S24] L. Liensberger, A. Kamra, H. Maier-Flaig, S. Geprägs, A. Erb, S. T. B. Goennenwein, R. Gross, W. Belzig, H. Huebl, and M. Weiler, Phys. Rev. Lett. **123**, 117204 (2019).
[S25] R. Cheng, S. Okamoto, and D. Xiao, Phys. Rev. Lett. **117**, 217202 (2016).
[S26] M. W. Daniels, R. Cheng, W. Yu, J. Xiao, and D. Xiao, Phys. Rev. B **98**, 134450 (2018).
[S27] J. Fabian, A. Matos-Abiague, C. Ertler, P. Stano, and I. Zutic, Acta Physica Slovaca **57**, 565 (2007).
[S28] A. Kamra, E. Thingstad, G. Rastelli, R. A. Duine, A. Brataas, W. Belzig, and A. Sudbø, Phys. Rev. B **100**, 174407 (2019).
